# Supplementary material for: Incremental Learning of Retrievable Skills For Efficient Continual Task Adaptation
Source: arXiv:2410.22658 source file (2025-01-21)
Supplement: Supplementary file 2 [file legacy.tex]

%% continual learning 방법론들의 장단 분석.
In continual imitation learning, various strategies have been proposed to overcome the challenges of preserving existing knowledge and assimilating new information within a single model, a process that necessitates the bidirectional knowledge transfer~\cite{rao2019continual}. These strategies are categorized as those in Figure~\ref{fig:fig0}. 
(a) \textbf{Rehearsal} approaches involve retaining a subset of previous data, to retrain the model periodically~\cite{chaudhry2019tiny, cril2021, schopf2022hypernetwork, Auddy2023ContinualLF, lotus2023}. While effective for knowledge retention, but these might not scale well due to high memory usages. They also often face data privacy issues. 
The others are rehearsal-free in that they do not retain previous data.
(b) \textbf{Weight regularization} approaches penalize changes to crucial model parameters learned from previous tasks~\cite{ewc2017}. Yet, fine-tuning the regularization parameters is considered challenging.
In the context of continual learning, pre-trained foundation models have been increasingly used, incorporating parameter efficient tuning (PET) methods. 
(c) \textbf{Sequential adaptation} approaches employ sequential updates of the pre-trained model via PET methods (e.g., adapters) for new tasks~\cite{liu2024tail}. The learning-to-modulate (L2M) method~\cite{l2m2023} addresses the adaptation capacity problem using low-rank adaptation (LoRA).   
(d) \textbf{Adapter matching} approaches use PET methods similar to (c), but with an emphasis on unsupervised adapter selection~\cite{rao2019continual, l2m2023, l2p2022, wang2022dualprompt}. 
%
% PEFT-based Continual Adaptation.
Still, these techniques have not been fully explored for bidirectional transfer, by which the model can improve not only on future tasks but also on those previously learned, due to the isolated nature of knowledge within individual adapters, each fine-tuned only within the confines of a single phase and its associated task.  % 당연한 이야기 to intro.

% To propose the (1) bidirectional transferable / (2) Unlearnable.
\color{red}
In this work, to propose the framework which satisfy these two property of lifelong learning, we adopt a similar approach to (d) the adapter marching approaches but hierarchical manner of skill-based knowledge management.
Distinct from the prior works that deal with clearly distinguishable states across multiple phases and typically extract task-specific knowledge in each phase in isolation, we take into account data streams from multiple phases that encompass overlapping sub-tasks. This perspective allows us to explore the bidirectional transfer capabilities using PET in a range of rehearsal-free continual imitation learning (RFCIL) scenarios. Our approach offers a more integrated and comprehensive RFCIL process in complex, long-horizon, dynamic environments, where tasks are subject to frequent variations and they often include shareable subtasks. 
\color{black}
% designed under assumption that tasks are easily distinguishable by input states. This assumption is not acceptable when data stream of dynamic multi-stage environments tasks encounterd, which often shares sub-tasks between tasks.
%
%Furthermore, in scenarios characterized by data scarcity and overlapping knowledge, methods like sequential-adaptation and adapter-matching often suffer from limited ability in backward knowledge transfer. % 이는 multi task 와 성능의 차이를 늘리게 되는...

\color{red}
To do so, we present \ours, a continual imitation learning unlearning framework designed to support the expansion of skills at each phase toward in-depth proficiency of individual skills and their broader coverage. 
In \ours, each data stream within a phase is decomposed and mapped to either skills previous learned or skill-complements, which are skills yet to be learned. Skill represent specific expert behavior patterns, derived from data streams, similar to~\cite{pertsch2020spirl}, and are encapsulated as policies to perform a series of actions upon specific states.
Skill-complements, on the other hand, are identified as gaps in the current skill set, representing new, unlearned behavior patterns that are essential for handling novel or unexplored situations. This decomposition facilitates both backward and forward transfer in the process of incremental skill learning in RFCIL.

%%%%%%%%% Evaluation %%%%%%%%%%%%%%%%
Our experiments demonstarte the ability of bidirectional knowledge transfer across various multi-stage and embodied environments.
\color{black}

% skill based policy of previous 
\subsection{Skill-based Policy} % Unsupervised skill learning // Knowledge Casting, Unsupervised 
Unsupervised skill discovery aims at finding a potentially useful set of skills without external rewards. For lifelong learning, these skills should both support maintain existing knowledge and make learning new skills.
% Formally, Markov decision process(MDP) defines $\mathcal{M} = (S,A,\mu,p)$ where $S$ and $A$ are state and action spaces, respectively, $\mu:P(S)$ is the initial state distribution. 
Each skill is defined as a skill latent vector $z \in Z$ and skill-conditioned policy $\pi(a|s,z)$ [that is shared across the skills]. The skill space $Z$ can be either discrete skills$\{1,...,D\}$ or continuous skills $R^D$ ~\cite{csd2023park}.
To collect a skill trajectory (behavior), we sample a skill z from a predefined skill prior distribution p(z) at the beginning of an episode. We then roll out the skill policy $\pi(a|s, z)$ with the sampled z for the entire episode. 
[TODO] For the skill prior, we use a standard normal distribution for continuous skills
and a uniform distribution for discrete skills.~\cite{csd2023park}

%%%%%%%%%%%%%%%%%%%%%%%%%%%%%%%%%%%%%%%%%%%%%%%%%%
%% 0505 related work 으로 갈 내용인듯
We introduce the Continual Imitation Learning and Unlearning framework (\ours), which incorporates bidirectional transfer to enhance sample efficiency and supports unlearning originating from task shifts in non-stationary environments and privacy concerns. Traditional continual imitation learning methods incrementally update task knowledge across the entire model, complicating unlearning \cite{bourtoule2021machine}. Moreover, existing unlearning techniques typically isolate the task knowledge in distinct parameters. These parameters are trained independently for removal, which is often impractical. This impracticality arises in scenarios where continuous learning is required, such as maintaining task boundary information during evaluations. Complete parameter isolation, common to both learning and unlearning, could establish strong baselines in this field \cite{liu2024tail, liu2022clpu}. However, this isolation method restricts knowledge sharing and still lowers data efficiency.
% 지속적인 모방 학습 및 언학습 프레임워크(\우리)를 소개합니다. 이 접근 방식은 지속적 모방 학습의 중요한 측면인 양방향 전이를 포괄하며, 언학습 단계의 성능을 해결합니다. 그러나 기존 지속적 모방 학습의 방식은 일반적으로 모델 내에서 작업 지식을 점진적으로 업데이트하기 때문에 언학습 과정이 복잡해집니다 \cite{bourtoule2021machine}. % 게다가 기존의 언러닝 기법은 일반적으로 독립적으로 학습된 모델 파라미터를 제거해야 하므로 평가 중에 작업 경계 정보를 유지해야 하는 등 지속적인 학습이 필요한 시나리오에서는 비현실적인 경우가 많습니다. % 학습과 비학습이 모두 공유하는 전략인 완전한 파라미터 격리를 활용하면 이 영역에서 강력한 프레임워크의 기반이 될 수 있습니다 \cite{liu2024tail, liu2022clpu}.% 하지만 이러한 격리 방식은 효과적인 지식 공유를제한하고 데이터 효율성을 떨어뜨립니다.
\ours consists of three parts to account for both characteristics 1) defines the skills that can be shared to perform a task and decouples the ability to combine skills from the ability to perform skills, 2) incrementally learns skills and the ability to combine skills, and 2-2) unlearns only the specific task by unlearning the ability to combine skills while preserving existing performance as much as possible. To decompose the abilities associated with skill composition and skill execution, we construct \ours with a goal-based two hierarchy with skills with marginal distributions. High-level policy $\pi_{hl}(z|o,\tau)$ estimate skill by observation and instruction. Low-level policy $\pi_{ll}(a|o,z)$ inference the action by conditioned skill. If the base model is already being used hierarchically, the policies can be extended as follows: $\pi_{hl}(g,z|o,\tau)$ for high-level $\pi_{ll}(a|o,g,z)$ for low-level where g is the output of the original high-level policy.
% \ours 이 두 가지 특성을 모두 고려하여 1) 작업 수행을 위해 공유할 수 있는 기술을 정의하고 기술을 결합하는 능력과 기술을 수행하는 능력을 분리하고, 2) 기술과 기술을 결합하는 능력을 점진적으로 학습하며, 3) 기존 성능을 최대한 보존하면서 기술을 결합하는 능력을 학습 해제하여 특정 작업만 학습 해제하는 세 부분으로 구성했습니다.
% Hierarchical skill decomposition 
% 만약, 이미 hierarchical 하게 사용되는 모델의 경우에는, HL 과 LL을 다음과 같이 extend 할 수 있다. $\pi_{hl}(g,z|o,\tau)$ $\pi_{ll}(a|o,g,z)$ where g is output original high-level policy.
% Sub-goal conditioned policy 0430
% 우리 실험에서, Multi-task Policy를 위해서 sub-goal conditioned pre-trained model(ICLR 2024)를 기본 모델 구조로 사용한다. (사전 학습되어있다) => Experiment에서 설명
%%%%%%%%%%%%%%%%%%%%%%%%%%%%%%%%%%%%%%%%%%%%%%%%%%%%%
0507 trash can

In each stage of CiL, the skill retriever $\Phi_Z$ involves an input-based prior $\SkillProto^{\text{pri}}$ and an output-based posterior $\SkillProto^{\text{post}}$ for a given demonstration.
%
%The skill retriever $\Phi_Z$ involves two types: an input-based prior $\SkillProto^{\text{pri}}$ and an output-based posterior $\SkillProto^{\text{post}}$. 
%Considering the multi-modal nature of expert behaviors,  
%$\Phi_Z$ is splited into two types: an input-based prior, $ \SkillProto^{\text{pri}} $, and an output-based posterior, $ \SkillProto^{\text{post}} $. 

The former retrieves skills that align with the input required by $\pi^{l}$ such as state $s$, while the latter classifies new skills and handles multi-modal behavioral skills by categorizing them based on the output of $\pi^{l}$ such as action $a$. We use an auxiliary threshold $\kappa_z$ for new skills, which is initialized by the median similarity score between the dataset used for initialize skill $z$ and behavior prototypes. 

During each phase of index $i$, we classify the novel skills ${z^*}$ and incorporate them into skills set $Z_{i} \leftarrow Z_{i-1} \cup \{z^*\}$ for adapter learning.
skill classification function $C(s, a)$ for early training stage is implemented using validity function $V(\hat{z}, s, a)$. 
\begin{equation}
     C(o, a) = \mathbb{I}[V(\hat{z}, o, a) = 1] \cdot \hat{z} + \mathbb{I}[V(\hat{z}, o, a) \neq 1] \cdot z^*
\end{equation}

% $C(s, a) = \hat{z} \text{ if } V(\hat{z}, s, a) = 1 \text{, else } z^*.$
% \begin{equation}
%     C(s,a) = \begin{cases}
%         \hat{z} & V(\hat{z},s,a) = 1, \\
%         z^*  & \text{otherwise}.
%         \end{cases}
% \end{equation}
For datasets that classify complementary parts of a skill in the current phase, a new skill $z^* \notin Z_{i-1} $ is initialized. $V(x, \hat{z})$ follows :
\begin{equation}
     V(\hat{z},o,a) = \mathbbm{1}(S(\chi_{\hat{z}}^{\text{pri}}, o) > \kappa^{\text{pri}}_{\hat{z}}) \cdot \mathbbm{1}(S(\chi_{\hat{z}}^\text{post}, a) > \kappa^{\text{post}}_{\hat{z}}) 
\end{equation}
where $\mathbbm{1}$ is an indicator function. If sub-goal information is available, the new skill $z^*$ for that phase can be divided into multiple skills, each corresponding to a sub-goal $g$.

Therefore, we address the novel problem in sequential decision making, the Continual Imitation Learning Unlearning (CiLU) problem. Similarly, in other classification fields, there are studies defining the problem of handling unlearning requests in continual learning scenarios, such as Learning with Selective Forgetting (LSF)\cite{shibata2021selec} and Continual Learning Private Unlearning (CLPU)\cite{liu2022clpu}. However, these studies have limited knowledge sharing ability or do not satisfy the assumptions for unlearning (weak unlearning). Therefore, in sequential decision making, it is challenging to use in multi-task non-stationary situations where shared skills must be utilized to enhance sample efficiency. Applying too strong negative learning (forgetting) to the unlearning task can degrade the generalization ability for unseen tasks and may hinder subsequent task learning.
% To do so, we address the novel problem in sequential decision making, the Continual Imitation Learning Unlearning (CiLU) problem. 
% Similarly 다른 Classification 분야에서 continual learning 시나리오에서 unlearning request를 handle하는 문제를 정의한 연구가 있다, Learning with Selective Forgetting(LSF)\cite{shibata2021selec},Continual Learning Private Unlearning CLPU\cite{liu2022clpu}.
% 하지만 위의 연구들은, limited knowledge sharing ability, or do not satisfy the assumptions for unlearning.(weak unlearning)
% 따라서, Sequential decision making 에서는, sample efficiency를 높이기 위해서 서로 공유되는 skill을 활용 해야하는 Multi-task non-stationary 상황에서 사용하기 힘들고, Unlearning task 에 대해 너무 강력한 negative learning(forgetting)을 적용하면 Unseen task에 대한 generarilzation 능력의 저하 및 추후 task 학습에 오히려 방해가 될 수 있어 사용하기 힘들다는 문제가 있다.

This scenario involves a continual learning process where it is also possible to forget tasks. This allows for the forgetting of knowledge about unnecessary tasks. Additionally, it must be capable of handling the unlearning of continual imitation learning due to personal information.
% 1. 해당 시나리오는 Continual 하게 배우는 과정에서 task의 망각 또한 수행이 가능한 시나리오이다.
% 1-2. 이는 불필요한 task에 대한 지식을 망각할 수 있다.
% 1-2. 개인정보로 인한 continual imitation learning unlearning을 처리 가능해야한다. 

\textbf{Continual Task Adaptation with pre-trained model.} 
% [Task Adaptation] 1. non-stationary tasks 2. efficiency on managing the tasks
% Pre-trained model adaptation and inaccurate matching.
Several recent works use pre-trained models, accumulating knowledge continually through additional Parameter Efficient Tuning (PET) modules such as adapters \cite{l2p2022, wang2022dualprompt, lae2023, codaprompt2023, huang2024ovor, l2m2023, color2023}. These methods enhance the flexibility and scalability of continual learning systems. However, they suffer from inaccurate matching between adapter selection and trained knowledge \cite{wang2022dualprompt, codaprompt2023}, which hinders overall performance.
% Decision making 에서의 문제.
In the realm of sequential decision making, some studies have explored adapting pre-trained models. For instance, \cite{l2m2023} assumes that the state space of tasks is completely separated, which limits its applicability in more integrated environments. Meanwhile, \cite{liu2024tail} requires comprehensive demonstrations for learning, which can be impractical in real-world scenarios.
%  LOTUS 와의 차별점. fixed state encoding or rehearsal. (Undo 불가능)
There are also studies that incorporate hierarchical structures in skill learning. The work by \cite{lotus2023} relies on rehearsal to mitigate knowledge loss but fails to completely resolve it.
% 우리의 방법들은
Our study aims to enhance task adaptation efficiency by using incrementally generalized skills with accurate matching on state space.
