# Supplementary material for: Incremental Learning of Retrievable Skills For Efficient Continual Task Adaptation
Source: arXiv:2410.22658 source file (2025-01-21)
Supplement: Supplementary file 4 [file Unseen.tex]

\begin{table}[h]
\begin{minipage}{.49\linewidth}
    \centering
    \caption{Evolving World-\textit{Complete} Unseen Tasks}
    \vskip 0.1 in
    \begin{adjustbox}{width=0.99 \columnwidth}
    \begin{tabular}{c|cccc}
    \toprule

    \multicolumn{5}{c}{\textbf{Evolving Kitchen-\textit{Complete}} Unseen}
    \midrule
    \textbf{Stage}
    & \multicolumn{1}{c}{\textbf{Sub-goal 1}}
    & \multicolumn{1}{c}{\textbf{Sub-goal 2}}
    & \multicolumn{1}{c}{\textbf{Sub-goal 3}}
    & \multicolumn{1}{c}{\textbf{Sub-goal 4}}\\

    \cmidrule(lr){1-5}
    
    5 & microwave & kettle & top burner & slide cabinet \\
    5 & microwave & kettle & top burner & top burner \\
    10 & microwave & kettle & top burner & light switch \\
    10 & kettle & bottom burner & top burner & light switch \\
    15 & kettle & top burner & slide cabinet & hinge cabinet \\
    15 & microwave & top burner & slide cabinet & hinge cabinet \\
    20 & microwave & top burner & light switch & slide cabinet \\
    20 & kettle & top burner & light switch & hinge cabinet \\
    \bottomrule
    \end{tabular}
    \end{adjustbox}
    \label{table:EK_unseen}
\end{minipage}
\hfill
\begin{minipage}{.49\linewidth}
    \centering
    \caption{Evolving World-\textit{Complete} unseen Tasks}
    \vskip 0.1 in
    \begin{adjustbox}{width=0.99 \columnwidth}
    \begin{tabular}{c|cccc}
    \toprule

    \multicolumn{5}{c}{\textbf{Evolving World-\textit{Complete} Unseen}}\\
    \midrule

    \textbf{Stage}
    & \multicolumn{1}{c}{\textbf{Sub-goal 1}}
    & \multicolumn{1}{c}{\textbf{Sub-goal 2}}
    & \multicolumn{1}{c}{\textbf{Sub-goal 3}}
    & \multicolumn{1}{c}{\textbf{Sub-goal 4}}\\

    \cmidrule(lr){1-5}
    
    handle-box-door-button & door & handle & button & box \\
    drawer-puck-stick-lever & puck & drawer & stick & lever \\
    door-handle-lever-puck & handle & puck & lever & door \\
    stick-drawer-box-button & button & drawer & box & stick \\
    button-handle-door-box & door & handle & box & button \\
    lever-puck-stick-drawer & puck & lever & drawer & stick \\
    lever-handle-puck-door & handle & lever & puck & door \\
    button-stick-drawer-box & box & drawer & stick & button \\
    handle-box-button-door & box & handle & door & button \\
    puck-stick-drawer-lever & lever & drawer & stick & puck \\
    door-lever-handle-puck & handle & lever & puck & door \\
    drawer-button-box-stick & box & drawer & stick & button \\
    button-door-handle-box & door & handle & box & button \\
    drawer-puck-lever-stick & puck & drawer & stick & lever \\
    puck-door-lever-handle & handle & puck & lever & door \\
    drawer-button-stick-box & box & drawer & stick & button \\
    door-button-handle-box & door & handle & box & button \\
    puck-lever-drawer-stick & lever & drawer & stick & puck \\
    puck-handle-door-lever & door & handle & lever & puck \\
    button-box-drawer-stick & box & drawer & stick & button \\
    \bottomrule
    \end{tabular}
    \end{adjustbox}
    \label{table:EW_unseen}
\end{minipage}
\end{table}
