# Supplementary material for: Incremental Learning of Retrievable Skills For Efficient Continual Task Adaptation
Source: arXiv:2410.22658 source file (2025-01-21)
Supplement: Supplementary file 5 [file baseline_table.tex]

\begin{table*}[t]
    \centering
    \caption{
    Baselines comparison
    }   
    \vskip 0.1 in
    \begin{adjustbox}{width=1.0 \textwidth}
    \begin{tabular}{l|ccccccccc}
    \toprule
    CL-algorithm
    & \metricc
    & \metricb
    & \metrica
    & \metricc
    & \metricb
    & \metrica
    & \metricc
    & \metricb
    & \metrica\\
    \midrule
    Pre-trained
    & 0.0{\color{gray}\scriptsize$\pm$0.0}
    & 0.0{\color{gray}\scriptsize$\pm$0.0}
    & 0.0{\color{gray}\scriptsize$\pm$0.0}
    & 0.0{\color{gray}\scriptsize$\pm$0.0}
    & 0.0{\color{gray}\scriptsize$\pm$0.0}
    & 0.0{\color{gray}\scriptsize$\pm$0.0}
    & 0.0{\color{gray}\scriptsize$\pm$0.0}
    & 0.0{\color{gray}\scriptsize$\pm$0.0}
    & 0.0{\color{gray}\scriptsize$\pm$0.0}
    \\
    \midrule
    Seq-FT
    & 0.0{\color{gray}\scriptsize$\pm$0.0}
    & 0.0{\color{gray}\scriptsize$\pm$0.0}
    & 0.0{\color{gray}\scriptsize$\pm$0.0}
    & 0.0{\color{gray}\scriptsize$\pm$0.0}
    & 0.0{\color{gray}\scriptsize$\pm$0.0}
    & 0.0{\color{gray}\scriptsize$\pm$0.0}
    & 0.0{\color{gray}\scriptsize$\pm$0.0}
    & 0.0{\color{gray}\scriptsize$\pm$0.0}
    & 0.0{\color{gray}\scriptsize$\pm$0.0}
    \\
    SPiRL-Seq
    & 0.0{\color{gray}\scriptsize$\pm$0.0}
    & 0.0{\color{gray}\scriptsize$\pm$0.0}
    & 0.0{\color{gray}\scriptsize$\pm$0.0}
    & 0.0{\color{gray}\scriptsize$\pm$0.0}
    & 0.0{\color{gray}\scriptsize$\pm$0.0}
    & 0.0{\color{gray}\scriptsize$\pm$0.0}
    & 0.0{\color{gray}\scriptsize$\pm$0.0}
    & 0.0{\color{gray}\scriptsize$\pm$0.0}
    & 0.0{\color{gray}\scriptsize$\pm$0.0}
    \\
    EWC(online)
    & 0.0{\color{gray}\scriptsize$\pm$0.0}
    & 0.0{\color{gray}\scriptsize$\pm$0.0}
    & 0.0{\color{gray}\scriptsize$\pm$0.0}
    & 0.0{\color{gray}\scriptsize$\pm$0.0}
    & 0.0{\color{gray}\scriptsize$\pm$0.0}
    & 0.0{\color{gray}\scriptsize$\pm$0.0}
    & 0.0{\color{gray}\scriptsize$\pm$0.0}
    & 0.0{\color{gray}\scriptsize$\pm$0.0}
    & 0.0{\color{gray}\scriptsize$\pm$0.0}
    \\
    Seq-LoRA
    & 0.0{\color{gray}\scriptsize$\pm$0.0}
    & 0.0{\color{gray}\scriptsize$\pm$0.0}
    & 0.0{\color{gray}\scriptsize$\pm$0.0}
    & 0.0{\color{gray}\scriptsize$\pm$0.0}
    & 0.0{\color{gray}\scriptsize$\pm$0.0}
    & 0.0{\color{gray}\scriptsize$\pm$0.0}
    & 0.0{\color{gray}\scriptsize$\pm$0.0}
    & 0.0{\color{gray}\scriptsize$\pm$0.0}
    & 0.0{\color{gray}\scriptsize$\pm$0.0}
    \\
    EWC-LoRA
    & 0.0{\color{gray}\scriptsize$\pm$0.0}
    & 0.0{\color{gray}\scriptsize$\pm$0.0}
    & 0.0{\color{gray}\scriptsize$\pm$0.0}
    & 0.0{\color{gray}\scriptsize$\pm$0.0}
    & 0.0{\color{gray}\scriptsize$\pm$0.0}
    & 0.0{\color{gray}\scriptsize$\pm$0.0}
    & 0.0{\color{gray}\scriptsize$\pm$0.0}
    & 0.0{\color{gray}\scriptsize$\pm$0.0}
    & 0.0{\color{gray}\scriptsize$\pm$0.0}
    \\
    \midrule
    L2M
    & 0.0{\color{gray}\scriptsize$\pm$0.0}
    & 0.0{\color{gray}\scriptsize$\pm$0.0}
    & 0.0{\color{gray}\scriptsize$\pm$0.0}
    & 0.0{\color{gray}\scriptsize$\pm$0.0}
    & 0.0{\color{gray}\scriptsize$\pm$0.0}
    & 0.0{\color{gray}\scriptsize$\pm$0.0}
    & 0.0{\color{gray}\scriptsize$\pm$0.0}
    & 0.0{\color{gray}\scriptsize$\pm$0.0}
    & 0.0{\color{gray}\scriptsize$\pm$0.0}
    \\
    L2M+TE
    & 0.0{\color{gray}\scriptsize$\pm$0.0}
    & 0.0{\color{gray}\scriptsize$\pm$0.0}
    & 0.0{\color{gray}\scriptsize$\pm$0.0}
    & 0.0{\color{gray}\scriptsize$\pm$0.0}
    & 0.0{\color{gray}\scriptsize$\pm$0.0}
    & 0.0{\color{gray}\scriptsize$\pm$0.0}
    & 0.0{\color{gray}\scriptsize$\pm$0.0}
    & 0.0{\color{gray}\scriptsize$\pm$0.0}
    & 0.0{\color{gray}\scriptsize$\pm$0.0}
    \\
    TAIL
    & 0.0{\color{gray}\scriptsize$\pm$0.0}
    & 0.0{\color{gray}\scriptsize$\pm$0.0}
    & 0.0{\color{gray}\scriptsize$\pm$0.0}
    & 0.0{\color{gray}\scriptsize$\pm$0.0}
    & 0.0{\color{gray}\scriptsize$\pm$0.0}
    & 0.0{\color{gray}\scriptsize$\pm$0.0}
    & 0.0{\color{gray}\scriptsize$\pm$0.0}
    & 0.0{\color{gray}\scriptsize$\pm$0.0}
    & 0.0{\color{gray}\scriptsize$\pm$0.0}
    \\
    \ours (ours)
    & 0.0{\color{gray}\scriptsize$\pm$0.0}
    & 0.0{\color{gray}\scriptsize$\pm$0.0}
    & 0.0{\color{gray}\scriptsize$\pm$0.0}
    & 0.0{\color{gray}\scriptsize$\pm$0.0}
    & 0.0{\color{gray}\scriptsize$\pm$0.0}
    & 0.0{\color{gray}\scriptsize$\pm$0.0}
    & 0.0{\color{gray}\scriptsize$\pm$0.0}
    & 0.0{\color{gray}\scriptsize$\pm$0.0}
    & 0.0{\color{gray}\scriptsize$\pm$0.0}
    \\
    \midrule
    Multi-task
    & 0.0{\color{gray}\scriptsize$\pm$0.0}
    & 0.0{\color{gray}\scriptsize$\pm$0.0}
    & 0.0{\color{gray}\scriptsize$\pm$0.0}
    & 0.0{\color{gray}\scriptsize$\pm$0.0}
    & 0.0{\color{gray}\scriptsize$\pm$0.0}
    & 0.0{\color{gray}\scriptsize$\pm$0.0}
    & 0.0{\color{gray}\scriptsize$\pm$0.0}
    & 0.0{\color{gray}\scriptsize$\pm$0.0}
    & 0.0{\color{gray}\scriptsize$\pm$0.0}
    \\
    \bottomrule
    \end{tabular}
    \end{adjustbox}
    \label{table:baselines}
    \vskip -0.1 in
\end{table*}
