# Supplementary material for: Incremental Learning of Retrievable Skills For Efficient Continual Task Adaptation
Source: arXiv:2410.22658 source file (2025-01-21)
Supplement: Supplementary file 6 [file dummy.tex]

\documentclass{article}
\usepackage{algorithm}
\usepackage{algorithmic}
\usepackage{lipsum}  % For generating dummy text

\usepackage{wrapfig}
\begin{document}

\lipsum[1]  % Dummy text

\begin{wrapfigure}{r}{0.5\textwidth}  % 오른쪽 정렬, 너비는 텍스트 너비의 50%
  \centering
      \begin{minipage}{\linewidth}
        \begin{flushright}
        \begin{algorithm}[H]  % The [H] here is to place the algorithm exactly here
        \caption{Example Algorithm}
        \begin{algorithmic}
        \STATE {Initialize the system}
        \FOR{$i=1$ to $N$}
        \STATE {Process the $i$-th element}
        \ENDFOR
        \STATE {Post-process results and output}
        \end{algorithmic}
        \end{algorithm}
        \end{flushright}
    \end{minipage}
\end{wrapfigure}

\lipsum[2-3]  % More dummy text

\end{document}
