# Supplementary material for: Incremental Learning of Retrievable Skills For Efficient Continual Task Adaptation
Source: arXiv:2410.22658 source file (2025-01-21)
Supplement: Supplementary file 7 [file icmla.tex]

\subsection{Detailed Experiment Settings and Metric}
To explore bidirectional transfer with skills and unlearning performance, we evaluate \ours in varying stream of demonstrations made up of multi-stage tasks.  

% In bidirectional transfer: backward trasfer 
\textbf{Evolving World. } 
%Evolving World is demonstration stream of multi-stage tasks which shares sub-task in Meta-world~\cite{yu2020meta,onis2023}. 
Evolving Wold is designed to emphasize backward transfer based on Meta-World environment~\cite{yu2020meta}. Especially, we leverage the data and environment proposed by  ~\cite{onis2023}. 
Each task comprises 4 out of 8 sub-tasks to solved sequentially. 
Evolving World-10 and Evolving World-20 are streams that differ in the number of phases based on task diversity. 
To investigate scenarios with limited data availability, we developed Evolving World-C. This version is a repeat of Evolving World-10, conducted twice. During each phase, sub-trajectories affected by a single sub-task are intentionally omitted to simulate data corruption. 
% 

% In bidirectional transfer: forwrard transer
\textbf{Evolving Kitchen. } 
Evolving Kitchen is designed to emphasize forward transfer based on Franka Kitchen tasks~\cite{fu2020d4rl, gupta2019relay}. 
%Evolving Kitchen is domain varying demonstration stream of Franka Kitchen tasks~\cite{fu2020d4rl,gupta2019relay}.
%
Each task comprises 4 out of 7 sub-tasks to solved sequentially. 
We have created three streams based on the diversity and extent of different domain tasks they comprise: Single, Mild, and Large. 
While all streams share the task configuration of each phase, the only difference is in the domain of each phase. 

\textbf{CL-ALFRED. } 
CL-ALFRED~\cite{kim2024alfcl} is embodied continual learning benchmark. 
%Evolving Kitchen is domain varying demonstration stream of Franka Kitchen tasks~\cite{fu2020d4rl,gupta2019relay}.
%
Each task comprises 4 out of 7 sub-tasks to solved sequentially. 
We have created three streams based on the diversity and extent of different domain tasks they comprise: Single, Mild, and Large. 
While all streams share the task configuration of each phase, the only difference is in the domain of each phase.

% where the domain difference is defined by characteristics of state distribution.~\cite{} % 0130

% \textbf{Pre-training. } We utilized diffusion model policy as outlined in~\cite{pearce2023imitating} to effectively utilize thier the adaptation ability ~\cite{ajay2023is, wang2023diffusion}. 
% %
% The base model for the Evolving World, which is trained on a single sub-task configuration, does not appear in the continual stream. The same applies to the Evolving Kitchen.
% % 
% In our experiments, all baselines used the same pre-trained base model for each environment.
% The details of environment settings and stream configurations are listed in Appendix. 

\textbf{Baselines. }
We compare our \ours with rehearsal-free baselines with two categories. (1) full-tuning approaches (2) parameter isolation and searching approach.
% \begin{comment}
Our experiment compares baselines with three categories. (1) Full-tuning approaches (2) PET-based accumulation approaches (3) Adapter-matching approaches. 
% (1)
(1) Full-tuning baselines, Sequential Fine-Tuning(\textbf{Seq-FT}) and Elastic Weight Consolidation (\textbf{EWC})~\cite{ewc2017} are commonly used rehearsal-free baselines in continual imitation learning. 
EWC stands out by using a regularization method to limit weight changes with previously learned model, effectively preserving past learning and reducing forgetting. 
EWC (L2) variants employ L2 regularization to preserve pre-trained knowledge.
% (2)
(2) PET-based accumulation baselines, \textbf{One Adapter} \cite{oneprompt2023} and \textbf{LAE}~\cite{lae2023} accumulate their knowledge on parameter of adapter, similar to full-tuning methods. However, LAE method often leading to unstable for evaluation in robotics task, we jointly optimize the training parameter with multi-task knowledge using~\cite{dylora2023}. for the acuumulation method, we set the adapter with a 64-rank low-rank adapter.
(3) Adapter matching-based baselines \textbf{L2M}~\cite{l2m2023} and \textbf{DACo+L2M}~\cite{dacorl2023} are State-of-the-Art continual learning baselines in robotics utilize the multiple adapters. 
 % progressive contextualization 
DACoRL requires context variable like trajectory information for adapter selection. We give single expert trajectory for context both training and evaluation for continual imitation learning setting.
For comparison, the adapter-pool for all adapter matching-based baselines and \ours, are consistently made up of 4-rank Low-Rank Adapters by default.
%\% 왜 phase-wise fine tuning이 oracle인지 납득 안됨, 실험이랑도 잘 안맞음 (oracle을 넘는 경우가 보임) 
% oracle 대신 사용할 것 있으면 이름 바꿔 치기, (없는듯)
In addition, \textbf{Oracle ID} (Phase-wise Adaptation)~\cite{liu2024tail} serves as the oracle baseline, and \textbf{Multi-task} learning, with full access to phase data, is served as the upper-bound of continual learning.
% \end{comment}
\textcolor{red}{How to set skill based policy as baseline? / 이거 그냥 Hierarchical policy 2개를 모두 Continual 하게 학습하는 방식인데... 이거 Seq는 Continual learning의 방식인데 그냥 이거를 Skill-based baseline 이라고 주장하는게 1번,  2번은 Pre-trained Skill policy 1개를 가지고 와서, low level의 continual learning없이 High level policy만 Continual learning 하고 unlearning 하는 방식을 비교군으로 가지고 오는 방식으로 설명을 해야될 것 같음.
즉 나머지의 continual learning 방식들은, Full model의 continual learning이라고 주장을 하고, skill-based는 option으로 추가된 방식이다.
정리하자면,1.  전체 비교군은 모델'전체'를 CLU 하는 방법, 2. 모델의 'high-level'만 continual learning 하는 skill-based learning 방식(가장 간단한 skill-based approach라고 주장)으로 크게 2가지로 나눠지며, 각 level에 적용하는 continual learning 방식이 달라질 뿐이다.  
}
\textcolor{green}{
\ours의 방법론들을 여러가지로 변경하도록 함. (Replay를 사용하는 경우 / 사용하지 않는 경우를 늘려가지고 전체 학습방식들을 비교해보자!
High level-supervised / Unsupervised
Low level-replay free / with Pesudo-replay
}

\section{Environment and Data Stream Details}
%\subsection{Detailed Stream Configuration}
%for each environment, state is constructed by concatnation of observation and language goal for sub-task. 

%--------------------------------------------------------------------------------------

% \begin{enumerate}
%     \item 목적: 이런 데이터셋을 만든 이유에 대한 설명
%     \item 행동: 데이터 구성간 차이점 설명
%     \item 구체적 내용: Table5를 이용한 dataset 구성 설명 / 해당 차이점이 어떤 결과를 이끌어 오는지 설명
    
% \end{enumerate}

% 해당 데이터셋은 Phase 개수에 따른 모델의 성능변화와, 모델의 BWT의 성능 평가를 위한 목적으로 설계되었다. 총 3가지 데이터셋이 존재하며, 각 데이터셋은 다른 특징을 가지고있다. Evolving World-10(10)을 기준으로 Evolving World-20(20)과 비교하면, Phase 개수에 따른 모델의 성능변화를 관찰할 수 있고, Evolving World-C(20)과 비교하면 모델의 BWT 성능 평가가 가능하다. 이런 특징을 가질 수 있도록, Sub-task를 구성했으며 그 결과는 Table(?) 이다.
\subsection{Evolving World}
Evolving World data stream was designed with two primary objectives: (1) to evaluate the changes in model performance with respect to the number of phases in terms of overall performance and forward transfer performance, and (2) to evaluate the impact on backward transfer performance by excluding certain sub-tasks. It consists of three distinct data streams, each characterized by different features. By comparing Evolving World-20(20) with Evolving World-10(10), one can observe the overall performance, forward transfer performance variations in models due to the number of pages. Additionally, comparing Evolving World-C(20) with Evolving World-10(10) enables the evaluation of model backward transfer performance. To facilitate these characteristics, sub-tasks were structured, and the results are presented in Table 

Evolving World-10 and Evolving World-20 are streams that differ in the number of phases based on task diversity. 
To investigate scenarios with limited data availability, we developed Evolving World-C. This version is a repeat of Evolving World-10, conducted twice. During each phase, sub-trajectories affected by a single sub-task are intentionally omitted to simulate data corruption. 

\ref{tab:tab5}.

\begin{table}[h]
    \centering
    \caption{Evolving World : Task and Sub-task Overview}
    \vskip 0.1 in
    \label{tab:table5}
    \begin{adjustbox}{width=0.48\textwidth}
        \centering
        \begin{tabular}{cc|cccc}
            \toprule[2pt]
    
            \multicolumn{6}{c}{\textbf{Evolving World-10(10)}}\\[5pt]
            
            \multicolumn{1}{c}{\textbf{Phase}} 
            & \multicolumn{1}{c}{\textbf{Task}} 
            & \multicolumn{1}{c}{\textbf{Sub-task 1}}
            & \multicolumn{1}{c}{\textbf{Sub-task 2}}
            & \multicolumn{1}{c}{\textbf{Sub-task 3}}
            & \multicolumn{1}{c}{\textbf{Sub-task 4}}\\

            \midrule
            \multirow{4}{*}{P1}
            & T1 & stick & handle & \textcolor{blue}{lever} & \textcolor{red}{box} \\
            & T2 & stick & handle & \textcolor{red}{box} & \textcolor{blue}{lever} \\
            & T3 & handle & \textcolor{blue}{lever} & \textcolor{red}{box} & stick \\
            & T4 & handle & \textcolor{blue}{lever} & stick & \textcolor{red}{box} \\
            \midrule
            \multirow{4}{*}{P2}
            & T5 & box & \textcolor{red}{handle} & door & \textcolor{blue}{button} \\
            & T6 & \textcolor{blue}{button} & door & \textcolor{red}{handle} & box \\
            & T7 & \textcolor{red}{handle} & door & \textcolor{blue}{button} & box \\
            & T8 & \textcolor{red}{handle} & \textcolor{blue}{button} & door & box \\
            \midrule
            \multirow{4}{*}{P3}
            & T9 & drawer & box & \textcolor{red}{lever} & stick \\
            & T10 & \textcolor{red}{lever} & box & drawer & stick \\
            & T11 & box & \textcolor{red}{lever} & stick & drawer \\
            & T12 & box & \textcolor{red}{lever} & drawer & stick \\
            \midrule
            \multirow{4}{*}{P4}
            & T13 & lever & handle & \textcolor{blue}{box} & door \\
            & T14 & door & lever & handle & \textcolor{blue}{box} \\
            & T15 & door & lever & \textcolor{blue}{box} & handle \\
            & T16 & door & \textcolor{blue}{box} & lever & handle \\
            \midrule
            \multirow{4}{*}{P5}
            & T17 & box & \textcolor{blue}{handle} & \textcolor{red}{button} & stick \\
            & T18 & box & \textcolor{blue}{handle} & stick & \textcolor{red}{button} \\
            & T19 & box & \textcolor{red}{button} & \textcolor{blue}{handle} & stick \\
            & T20 & stick & \textcolor{blue}{handle} & \textcolor{red}{button} & box \\
            \midrule
            \multirow{4}{*}{P6}
            & T21 & \textcolor{blue}{drawer} & box & \textcolor{red}{door} & lever \\
            & T22 & lever & \textcolor{blue}{drawer} & \textcolor{red}{door} & box \\
            & T23 & box & \textcolor{red}{door} & lever & \textcolor{blue}{drawer} \\
            & T24 & box & \textcolor{red}{door} & \textcolor{blue}{drawer} & lever \\
            \midrule
            \multirow{4}{*}{P7}
            & T25 & \textcolor{red}{drawer} & stick & \textcolor{blue}{button} & box \\
            & T26 & \textcolor{blue}{button} & box & \textcolor{red}{drawer} & stick \\
            & T27 & \textcolor{blue}{button} & stick & box & \textcolor{red}{drawer} \\
            & T28 & stick & box & \textcolor{blue}{button} & \textcolor{red}{drawer} \\
            \midrule
            \multirow{4}{*}{P8}
            & T29 & lever & \textcolor{red}{puck} & \textcolor{blue}{stick} & handle \\
            & T30 & \textcolor{red}{puck} & lever & handle & \textcolor{blue}{stick} \\
            & T31 & \textcolor{blue}{stick} & \textcolor{red}{puck} & handle & lever \\
            & T32 & lever & handle & \textcolor{blue}{stick} & \textcolor{red}{puck} \\
            \midrule
            \multirow{4}{*}{P9}
            & T33 & button & \textcolor{red}{box} & drawer & \textcolor{blue}{door} \\
            & T34 & \textcolor{blue}{door} & \textcolor{red}{box} & drawer & button \\
            & T35 & button & \textcolor{red}{box} & \textcolor{blue}{door} & drawer \\
            & T36 & \textcolor{red}{box} & drawer & button & \textcolor{blue}{door} \\
            \midrule
            \multirow{4}{*}{P10}
            & T37 & \textcolor{blue}{lever} & door & puck & \textcolor{red}{handle} \\
            & T38 & puck & \textcolor{red}{handle} & door & \textcolor{blue}{lever} \\
            & T39 & \textcolor{red}{handle} & puck & \textcolor{blue}{lever} & door \\
            & T40 & door & puck & \textcolor{blue}{lever} & \textcolor{red}{handle} \\
        
            \bottomrule[2pt]
        \end{tabular}
    \end{adjustbox}%
    \hspace{1cm}
    \begin{adjustbox}{width=0.44\textwidth}
        \centering
        \begin{tabular}{cc|cccc}
            \toprule[2pt]
            
            \multicolumn{6}{c}{\textbf{Evolving World-20(20)}}\\[5pt]
            
            \multicolumn{1}{c}{\textbf{Phase}} 
            & \multicolumn{1}{c}{\textbf{Task}} 
            & \multicolumn{1}{c}{\textbf{Sub-task 1}}
            & \multicolumn{1}{c}{\textbf{Sub-task 2}}
            & \multicolumn{1}{c}{\textbf{Sub-task 3}}
            & \multicolumn{1}{c}{\textbf{Sub-task 4}}\\
        
            \midrule
            
            \multirow{2}{*}{P1}
            & T1 & stick & handle & lever & box \\
            & T2 & stick & handle & box & lever \\
            \midrule
            \multirow{2}{*}{P2}            
            & T3 & box & handle & door & button \\
            & T4 & button & door & handle & box \\
            \midrule
            \multirow{2}{*}{P3}
            & T5 & drawer & box & lever & stick \\
            & T6 & lever & box & drawer & stick \\
            \midrule
            \multirow{2}{*}{P4}
            & T7 & lever & handle & box & door \\
            & T8 & door & lever & handle & box \\
            \midrule
            \multirow{2}{*}{P5}
            & T9 & box & handle & button & stick \\
            & T10 & box & handle & stick & button \\
            \midrule
            \multirow{2}{*}{P6}
            & T11 & drawer & box & door & lever \\
            & T12 & lever & drawer & door & box \\
            \midrule
            \multirow{2}{*}{P7}
            & T13 & drawer & stick & button & box \\
            & T14 & button & box & drawer & stick \\
            \midrule
            \multirow{2}{*}{P8}
            & T15 & lever & puck & stick & handle \\
            & T16 & puck & lever & handle & stick \\
            \midrule
            \multirow{2}{*}{P9}
            & T17 & button & box & drawer & door \\
            & T18 & door & box & drawer & button \\
            \midrule
            \multirow{2}{*}{P10}
            & T19 & lever & door & puck & handle \\
            & T20 & puck & handle & door & lever \\
            \midrule
            \multirow{2}{*}{P11}
            & T21 & handle & stick & button & puck \\
            & T22 & puck & handle & stick & button \\
            \midrule
            \multirow{2}{*}{P12}
            & T23 & stick & lever & puck & drawer \\
            & T24 & puck & drawer & lever & stick \\
            \midrule
            \multirow{2}{*}{P13}
            & T25 & button & puck & handle & door \\
            & T26 & button & door & puck & handle \\
            \midrule
            \multirow{2}{*}{P14}
            & T27 & puck & door & lever & drawer \\
            & T28 & lever & drawer & door & puck \\
            \midrule
            \multirow{2}{*}{P15}
            & T29 & drawer & puck & stick & button \\
            & T30 & button & stick & puck & drawer \\
            \midrule
            \multirow{2}{*}{P16}
            & T31 & handle & box & button & stick \\
            & T32 & button & stick & box & handle \\
            \midrule
            \multirow{2}{*}{P17}
            & T33 & button & drawer & box & door \\
            & T34 & button & drawer & door & box \\
            \midrule
            \multirow{2}{*}{P18}
            & T35 & puck & button & door & handle \\
            & T36 & button & puck & handle & door \\
            \midrule
            \multirow{2}{*}{P19}
            & T37 & lever & stick & handle & puck \\
            & T38 & puck & handle & lever & stick \\
            \midrule
            \multirow{2}{*}{P20}
            & T39 & box & handle & lever & door \\
            & T40 & handle & door & lever & box \\
            
            \bottomrule[2pt]
        \end{tabular}
    \end{adjustbox}
    \label{tab:tab5}
\end{table}

The composition of the three data streams is as follows:
\begin{enumerate}
    \item Evolving World-10(10): This data stream is composed of a total of 40 tasks, each task is divided into 4 distinct sub-tasks. It is organized into 10 phases, with each containing 4 similar tasks.
    \item Evolving World-20(20): This data stream is composed of a total of 40 tasks, each task is divided into 4 distinct sub-tasks. It is organized into 20 phases, with each containing 2 similar tasks.
    \item Evolving World-C(20): This data stream is composed of a total of 40 tasks, each task is divided into 3~4 distinct sub-tasks. It is organized into 20 phases, with each containing 4 similar tasks. It represents a repeated structure of Evolving World-10(10) with a twist: certain sub-tasks are excluded on each phase. The first iteration excludes sub-tasks highlighted in red in Table \ref{tab:tab5}, while the second iteration excludes those marked in blue.
\end{enumerate}
Refer to Figure \ref{fig:fig5} for a clearer understanding of the data stream's composition. This figure visualizes the features of each task in both Evolving World-10(10) and Evolving World-20(20). It reveals groups of similar tasks, with 4 tasks in one group and 2 in another.

\begin{figure*}[h]
    \centering
    \begin{minipage}{.48\textwidth}
        \centering
        \includegraphics[width=\linewidth]{icml2024/graphs/world_mean_first.pdf}
    \end{minipage}% 
    \begin{minipage}{.48\textwidth}
        \centering
        \includegraphics[width=\linewidth]{icml2024/graphs/world_mean_second.pdf}
    \end{minipage}
    \caption{Evolving World : State Feature Comparison}
    \label{fig:fig5}
\end{figure*}

\subsection{Evolving Kitchen}
The data stream under consideration is structured into a total of 24 distinct tasks, with each task further subdivided into four sub-tasks. The sub-tasks included in each task follow the same order as in the Table \ref{table:appendix1}.

\begin{table*}[h]
    \centering
    \caption{Evolving Kitchen : Task and Sub-task Overview}
    \vskip 0.1 in
    \begin{adjustbox}{width=0.5 \textwidth}
    \begin{tabular}{l|cccc}
    \toprule[2pt]

    \multicolumn{5}{c}{\textbf{Evolving Kitchen}}\\[5pt]
    
    \multicolumn{1}{l}{\textbf{Task}} 
    & \multicolumn{1}{c}{\textbf{Sub-task 1}}
    & \multicolumn{1}{c}{\textbf{Sub-task 2}}
    & \multicolumn{1}{c}{\textbf{Sub-task 3}}
    & \multicolumn{1}{c}{\textbf{Sub-task 4}}\\

    \cmidrule(lr){1-5}
    
    T1 & bottom burner & top burner & slide cabinet & hinge cabinet \\
    T2 & kettle & bottom burner & top burner & light switch \\
    T3 & bottom burner & top burner & light switch & slide cabinet \\
    T4 & kettle & bottom burner & slide cabinet & hinge cabinet \\
    T5 & microwave & light switch & slide cabinet & hinge cabinet \\
    T6 & microwave & kettle & slide cabinet & hinge cabinet \\
    T7 & microwave & bottom burner & slide cabinet & hinge cabinet \\
    T8 & kettle & light switch & slide cabinet & hinge cabinet \\
    T9 & kettle & top burner & light switch & slide cabinet \\
    T10 & kettle & bottom burner & light switch & slide cabinet \\
    T11 & microwave & top burner & light switch & hinge cabinet \\
    T12 & microwave & kettle & bottom burner & hinge cabinet \\
    T13 & microwave & kettle & top burner & hinge cabinet \\
    T14 & microwave & bottom burner & light switch & slide cabinet \\
    T15 & kettle & bottom burner & light switch & hinge cabinet \\
    T16 & microwave & kettle & top burner & light switch \\
    T17 & microwave & bottom burner & top burner & slide cabinet \\
    T18 & microwave & kettle & bottom burner & slide cabinet \\
    T19 & microwave & bottom burner & top burner & light switch \\
    T20 & kettle & bottom burner & top burner & hinge cabinet \\
    T21 & microwave & kettle & light switch & hinge cabinet \\
    T22 & microwave & kettle & light switch & slide cabinet \\
    T23 & kettle & bottom burner & top burner & slide cabinet \\
    T24 & microwave & bottom burner & top burner & hinge cabinet \\
    
    \bottomrule[2pt]
    \end{tabular}
    \end{adjustbox}
    \label{table:appendix1}
\end{table*}
% \begin{enumerate}
%     \item 상황: task 간의 변화가 크지 않아서, task 간의 도메인 결과를 크게 만들겠다. 
% \end{enumerate}
An analysis of the results indicates minimal variance in the similarity across tasks. To address this, we introduced changes in the domain by applying a scale factor to the original state values and incorporating a shift value, thus altering the distributions. 
This methodology facilitated the development of three data streams, each characterized by distinct state distributions among tasks. 
The specific scale and shift parameters employed for each domain are detailed in Figure \ref{fig:fig5}.

% \begin{enumerate}
%     \item 목적: the purpose of analyzing the dataset
%     \item 행동: We compute JS-divergence 
%     \item 구체적 내용: under assumption that states follows normal distribution
% \end{enumerate}

To analyze the domain difference between data streams, we calculate the Jensen-Shannon (JS) divergence among tasks, under assumption that states of each task follow the normal distribution. This is not true, but enough to estimate the differences among tasks. The results  are presented in Figure \ref{fig:fig6}. 

The domain configurations for the three data streams are described as follows:
\begin{enumerate}
    \item Evolving Kitchen-Single(24): This data stream is a single domain, using only domain1. The results of domain1 are the same as the original data stream analyzed earlier.
    \item   Evolving Kitchen-Mild(24): This data stream uses two domains: domain1 and domain2. It alternates between domain1 and domain2 for each task, for instance, Task 1 uses domain1, Task 2 uses domain2, Task 3 uses domain1, and so on.
    \item  Evolving Kitchen-Large(24): This data stream uses four domains: domain1, domain2, domain3, and domain4. sequentially alternating among domain1, domain2, domain3, and domain4 for each Task, for instance, Task 1 uses domain1, Task 2 uses domain2, Task 3 uses domain3, Task 4 uses domain4, Task 5 uses domain1, and so on.
\end{enumerate}
 
As demonstrated in Figure \ref{fig:fig6}, the JS divergence allows for the observation of similarity changes among tasks across three data streams generated due to domain variation.

\section{Metrics}
We report 4 metrics for learning and unlearning performance for tasks: Forward Transfer(FWT), Backward Transfer(BWT), Area Under Curve(AUC) and Forgetting(FGT)\cite{liu2023libero, liu2024tail}. 
In multi-stage environment task, we report performance using the Goal Conditioned(GC) success rates, that evaluates the average success rate of successfully completed sub-goals out of $N$ sub-goals\cite{shridhar2020alfred}.
For Learning performance FWT, BWT, AUC are used and For Unlearning performance FGT is used.
\begin{itemize}
    \item \textbf{FWT}: $FWT_k =  C_{k}$ where $K$ is phase id and $C_{k}$ represents the average score tasks occurence in the phase $k$. 
    \item \textbf{BWT}: $BWT_k = \frac{1}{P - p} \sum_{\tau=p+1}^{P} (C_{\tau,k}-C_{k}).$, where $P$ is final phase(or final phase number of task unlearned) and $p$ is phase the task $t$ first appeared. $C_{\tau,k}$ is the performance of task of phase $k$ in current phase $\tau$. 
    \item \textbf{AUC}: $AUC_k = \frac{1}{P - p + 1} ( FWT_k + \sum_{\tau=p+1}^{P} C_{\tau,k})$, represent the the overall performance of continual learning, balancing FWT and BWT.
    \item \textbf{FGT}: $FGT_k = \frac{1}{U - p} \sum_{\tau=p+1}^{U} (C_{k}-C_{\tau,k})$, where $U$ is unlearning phase of target task and $p$ is phase the task $t$ first appeared. $C_{\tau,k}$ is the performance of task $k$ in phase $\tau$. 
    $FGT_k = \sum_{p}^{U} AUC - \sum_{U}^{P}$
\end{itemize}
For all metrics, we use the average of all learned tasks for reporting, with higher values indicating better performance.

\section{Implementation Details}
\subsection{Pre-trained Model Configure}
For pre-trained model, we implement a diffusion-based policy.
\begin{table}[h]
    \centering
    \caption{Pre-trained model configure}   
    \vskip 0.1 in
    \begin{adjustbox}{width=0.3 \columnwidth }
    \begin{tabular}{l|c}
    \toprule
    
    \multicolumn{1}{c}{\textbf{Hyperparameter}}
    & \multicolumn{1}{c}{Value}\\
    \midrule
    Diffusion Model & DDPM~\cite{2020ddpm}\\
    Denoising step & 32\\
    \midrule 

    Block & MLP \\
    The number of layers & 6 \\
    hidden dimension & 512 \\
    Schedule & Linear \\
    Linear start & 1e-4 \\
    Linear end & 1e-2 \\
        \bottomrule
    \end{tabular}
    \end{adjustbox}
    \label{table:ablation}
    \vskip -0.1 in
    
\end{table}

\begin{table*}[h]
    \centering
    \caption{Evolving Kitchen Pre-trained Model: Task and Sub-task Overview}
    \vskip 0.1 in
    \begin{adjustbox}{width=0.5 \textwidth}
    \begin{tabular}{l|cccc}
    \toprule[2pt]

    \multicolumn{5}{c}{\textbf{Evolving Kitchen Pre-trained Model}}\\[5pt]
    
    \multicolumn{1}{l}{\textbf{Task}} 
    & \multicolumn{1}{c}{\textbf{Sub-task 1}}
    & \multicolumn{1}{c}{\textbf{Sub-task 2}}
    & \multicolumn{1}{c}{\textbf{Sub-task 3}}
    & \multicolumn{1}{c}{\textbf{Sub-task 4}}\\

    \cmidrule(lr){1-5}
    
    T1 & bottom burner & top burner & - & - \\
    T2 & kettle & bottom burner & top burner & light switch \\
    T3 & bottom burner & top burner & light switch & - \\
    T4 & kettle & bottom burner & - & - \\
    T5 & kettle & light switch & - & - \\
    T6 & kettle & top burner & light switch & - \\
    T7 & kettle & bottom burner & light switch & - \\
    T8 & kettle & bottom burner & light switch & - \\
    T9 & kettle & bottom burner & top burner & - \\
    T10 & kettle & bottom burner & top burner & - \\

    \bottomrule[2pt]
    \end{tabular}
    \end{adjustbox}
    \label{table:appendix1}
\end{table*}

\begin{table*}[h]
    \centering
    \caption{Evolving World Pre-trained Model: Task and Sub-task Overview}
    \vskip 0.1 in
    \begin{adjustbox}{width=0.5 \textwidth}
    \begin{tabular}{l|cccc}
    \toprule[2pt]

    \multicolumn{5}{c}{\textbf{Evolving World Pre-trained Model}}\\[5pt]
    
    \multicolumn{1}{l}{\textbf{Task}} 
    & \multicolumn{1}{c}{\textbf{Sub-task 1}}
    & \multicolumn{1}{c}{\textbf{Sub-task 2}}
    & \multicolumn{1}{c}{\textbf{Sub-task 3}}
    & \multicolumn{1}{c}{\textbf{Sub-task 4}}\\

    \cmidrule(lr){1-5}
    
    T1 & drawer & puck & door & button \\
    T2 & door & puck & button & drawer \\
    T3 & door & puck & drawer & button \\
    T4 & door & button & puck & drawer \\
    T5 & button & drawer & door & puck \\
    T6 & door & drawer & button & puck \\
    T7 & button & drawer & puck & door \\
    T8 & drawer & door & puck & button \\
    T9 & puck & drawer & door & button \\
    T10 & button & puck & door & drawer \\
    T11 & drawer & button & door & puck \\
    T12 & door & button & drawer & puck \\
    T13 & drawer & button & puck & door \\
    T14 & button & door & drawer & puck \\
    T15 & door & drawer & puck & button \\
    T16 & puck & button & door & drawer \\
    T17 & drawer & door & button & puck \\
    T18 & puck & drawer & button & door \\
    T19 & button & door & puck & drawer \\
    T20 & puck & button & drawer & door \\
    T21 & button & puck & drawer & door \\
    T22 & puck & door & button & drawer \\
    T23 & puck & door & drawer & button \\
    T24 & drawer & puck & button & door \\

    \bottomrule[2pt]
    \end{tabular}
    \end{adjustbox}
    \label{table:appendix1}
\end{table*}

\begin{table}[h]
    \centering
    \caption{Pre-trained model performance}   
    \vskip 0.1 in
    \begin{adjustbox}{width=1\columnwidth }
    \begin{tabular}{c|c|ccc}
    \toprule
    \textbf{Stream}(Total phase)
    & Evolving World Base
    & \multicolumn{1}{c}{Evolving World-10(10)}
    & \multicolumn{1}{c}{Evolving World-20(20)}
    & \multicolumn{1}{c}{Evolving World-C(20)}
    \\
    \midrule
    Evolving World Pre-trained
    & 98.3{\color{gray}\scriptsize$\pm$1.26}
    & 7.0{\color{gray}\scriptsize$\pm$0.4}
    & 11.9{\color{gray}\scriptsize$\pm$0.3}
    & 7.0{\color{gray}\scriptsize$\pm$0.4}\\
    \midrule
    \textbf{Stream}(Total phase)
    & Evolving Kitchen base
    & \multicolumn{1}{c}{Evolving Kitchen-Single(24)}
    & \multicolumn{1}{c}{Evolving Kitchen-Mild(24)}
    & \multicolumn{1}{c}{Evolving Kitchen-Large(24)}\\
    \midrule
    Evolving Kitchen Pre-trained
    & 91.3{\color{gray}\scriptsize$\pm$8.8}
    & 28.8{\color{gray}\scriptsize$\pm$0.4}
    & 15.6{\color{gray}\scriptsize$\pm$0.6}
    & 5.7{\color{gray}\scriptsize$\pm$0.5}\\
    
    \midrule
    
    % & \multicolumn{3}{c}{Evolving Kitchen(24)}\\
    
    % \cmidrule(lr){1-2}
    % \cmidrule(lr){3-5}
    
    % Baselines& rehearsal
    % & \metricc
    % & \metricb
    % & \metrica \\

    % \multirow{4}{*}{ER}&  50
    % & 85.0{\color{gray}\scriptsize$\pm$3.3}
    % & -37.8{\color{gray}\scriptsize$\pm$2.3}
    % & 51.7{\color{gray}\scriptsize$\pm$1.5}\\
    
    % & 100
    % & 82.8{\color{gray}\scriptsize$\pm$1.5}
    % & -31.3{\color{gray}\scriptsize$\pm$4.5}
    % & 55.0{\color{gray}\scriptsize$\pm$2.8}\\

    % & 500
    % & 82.3{\color{gray}\scriptsize$\pm$2.5}
    % & -15.0{\color{gray}\scriptsize$\pm$3.3}
    % & 66.0{\color{gray}\scriptsize$\pm$0.3}\\
    
    % & 1000
    % & 81.5{\color{gray}\scriptsize$\pm$1.5}
    % & -10.3{\color{gray}\scriptsize$\pm$2.8}
    % & 72.0{\color{gray}\scriptsize$\pm$1.5}\\
    % \midrule
    
    % \ours & 0
    % & 88.5{\color{gray}\scriptsize$\pm$3.0}
    % & -3.0{\color{gray}\scriptsize$\pm$3.0}
    % & 85.5{\color{gray}\scriptsize$\pm$0.3}\\

    % \bottomrule
    \end{tabular}
    \end{adjustbox}
    \label{table:pre-trained}
    \vskip -0.1 in
    
\end{table}

%\subsection{Modulator Configuration}

% \subsection{Modulator Arithmetic} 
% define modulator summation and BWT,FWT modular combination.

% \subsection{Metrics Details}
% Here, introduces specific information on indicators to evaluate continual learing performance.
% \begin{itemize}
%     \item AUC : 
%     \item FGT :
%     \item FWT :
% \end{itemize}

% \subsection{Baseline Implementation}
% \textbf{One Modulator. }
% \textbf{LAE. }
% \textbf{L2M. }
% \textbf{DACORL+LoRA. }
% \textbf{CODA+L2M. }

% \section{Extended Experimental results}
% this section shows extended experimental results 

\section{More Details}
\subsection{Machine Unlearning}
% [1] What is Unlearning 
Machine unlearning aims to minimize the influence of a target unlearning task dataset $D_f$ from the entire dataset to a model trained with $D$.
Specifically, it aims to generate a model that is indistinguishable from the one learned from the rest of the set $D_r = D \setminus D_f$ alone where $\setminus$ denotes set minus operation. The strong unlearning follows the formula 
\begin{equation}
\forall D, \, \text{if } D_f \subseteq D, \text{ then } A(D_r) {=}_d R_A(D, A(D), D_f).
\end{equation}
Here, $A(D \setminus D_f)$ represents the distribution of model parameters learned by algorithm $A$ after the subset $D_f$ is removed from $D$. $R_A(D, A(D), D_f)$ denotes the distribution of model parameters following the application of the unlearning algorithm $R_A$ on $D$. The symbol ${=}_d$ indicates distributional equivalence.
% [2] Type of Unlearning / What is Task Unleanring in imitation learning
However, while exact unlearning can completely eliminate certain samples, it is quite restrictive. 
Therefore, a looser condition for removing the target dataset while maximizing overall model performance, weak unlearning aims to unlearn the overall behavior of the model as measured by the model's output distribution or task performance. 
% [3] output distribution indistringuishable/approximated unlearning
only output distributional equivalence between the remained dataset and the unlearned model evaluated.
specifically, weak unlearning follows
\begin{equation}
\forall D, \, \text{if } D_f \subseteq D, \text{ then } O (A(D_r) , D_r) \quad {=}_d \quad O (R_A(D, A(D), D_f), D_r).
\end{equation}
$O$ is a function that uses model parameters derived from a dataset and a learning algorithm to produce results or inferences.
